# Supplementary material for: NTTSuite: Number Theoretic Transform Benchmarks for Accelerating Encrypted Computation
Source: arXiv:2405.11353 source file (2024-05-18)
Supplement: Supplementary file 1 [file Appendix.tex]

\section{Appendix}
\setcounter{figure}{1} 
\setcounter{table}{0} 

% \begin{figure*}[htbp]
%     \centerline{\includegraphics{plots/optm_methodspng.png}}
%     \caption{Optimization Methods}
%     \label{fig:Optimization Methods}
% \end{figure*}

% \begin{figure*}[htbp]
%     \centering
%     \includegraphics[width=\textwidth]{plots/1024 points Accleration.png}
%     \includegraphics[width=\textwidth]{plots/4096 points Accleration.png}
%     \includegraphics[width=\textwidth]{plots/16384 points Accleration.png}
%     \caption{Acceleration on FPGA and GPU}
%     \label{fig:Acceleration}
% \end{figure*}
